# Supplementary material for: Diversity and Disorder in the Voter Model with Delays
Source: arXiv:1708.08756 ancillary file (2017-09-19)
Supplement: Supplementary file 1 [file supplemental.pdf]

# Diversity and Disorder in the Voter Model with Delays

## Supplemental Material

## 1 Supplemental Graphs

The addition of delays in the voter model causes opinion coexistence by limiting the sizes of domains having the same opinion, which shows up in simulations as the correlation lenght reaching a maximum value. The dependence of these domain sizes is illustrated by the snapshots of the lattice found in figure 1

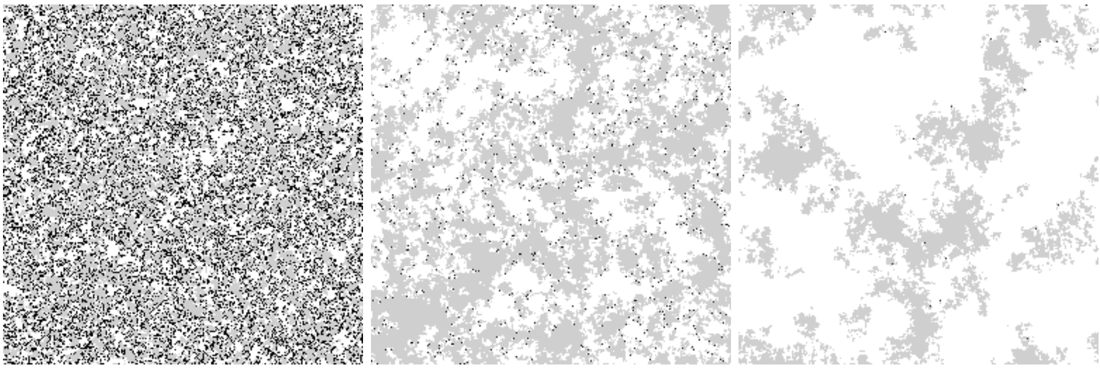

(a) $\lambda = 1$ (b) $\lambda = 2^4$ (c) $\lambda = 2^8$

Figure 1: Lattice snapshots for $M = 2$, $L = 256$ and $\lambda = 1, 2^4$ and $2^8$. White pixels represent non-susceptibles with opinion 1, gray pixels represent non-susceptibles with opinion 2 and black pixels represent susceptibles (of both opinions)

The remainder of the graphs of $\log\left(\frac{L\sigma}{\sqrt{\lambda}}\right)$ by $\log\left(\frac{t}{\lambda L^2}\right)$ (complementing figure 3 of the main article) can be found in figures 2 to 6

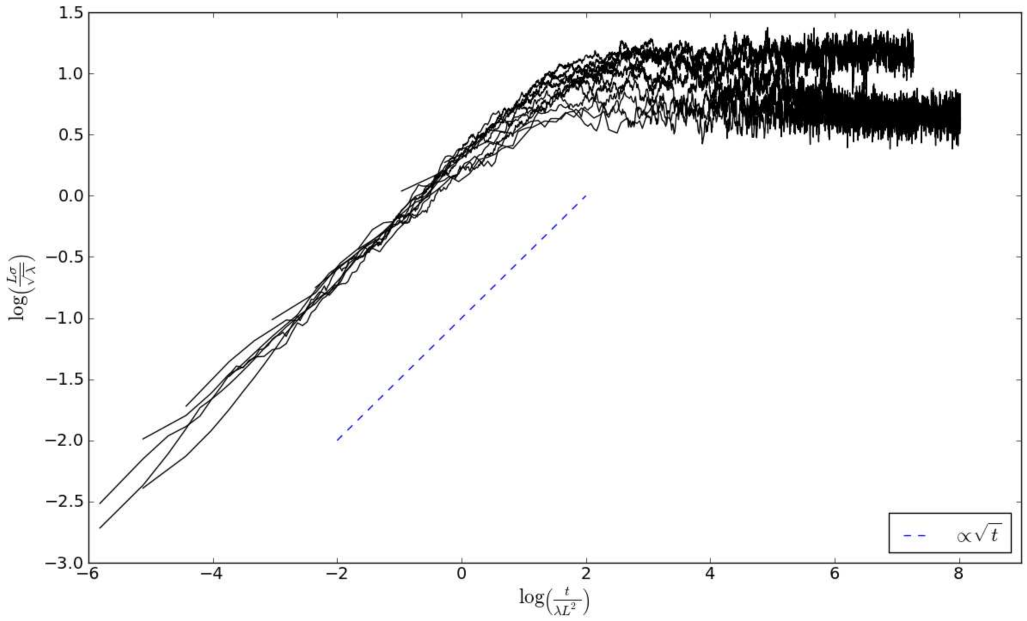


Figure 2: Graph of $\log\left(\frac{L\sigma}{\sqrt{\lambda}}\right)$ by $\log\left(\frac{t}{\lambda L^2}\right)$ for $M = 2$ and $L$ ranging from 32 to 512.

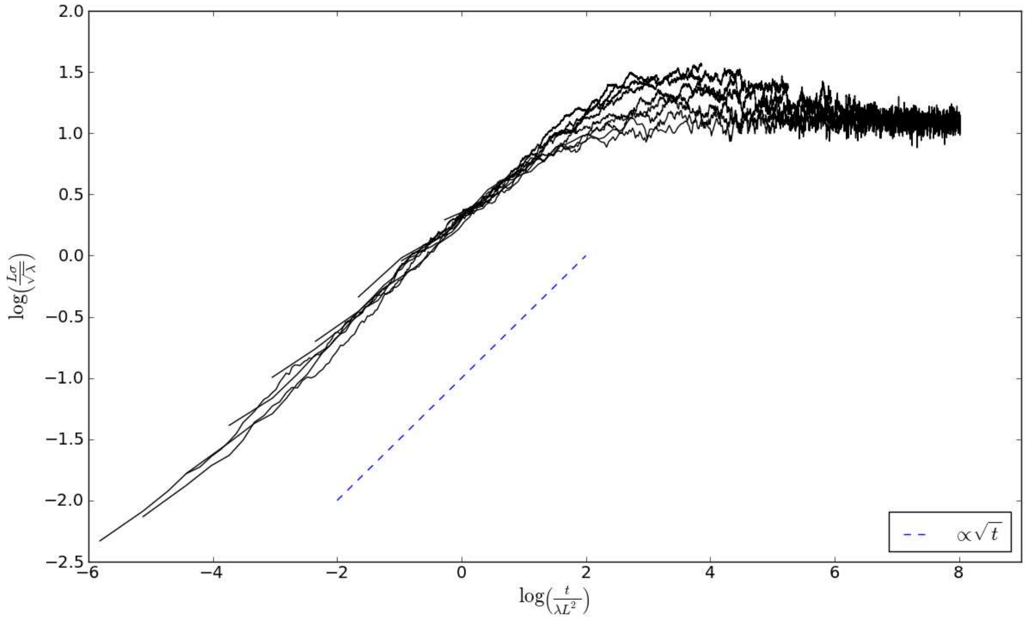


Figure 3: Graph of $\log\left(\frac{L\sigma}{\sqrt{\lambda}}\right)$ by $\log\left(\frac{t}{\lambda L^2}\right)$ for $M = 3$ and $L$ ranging from 32 to 256.

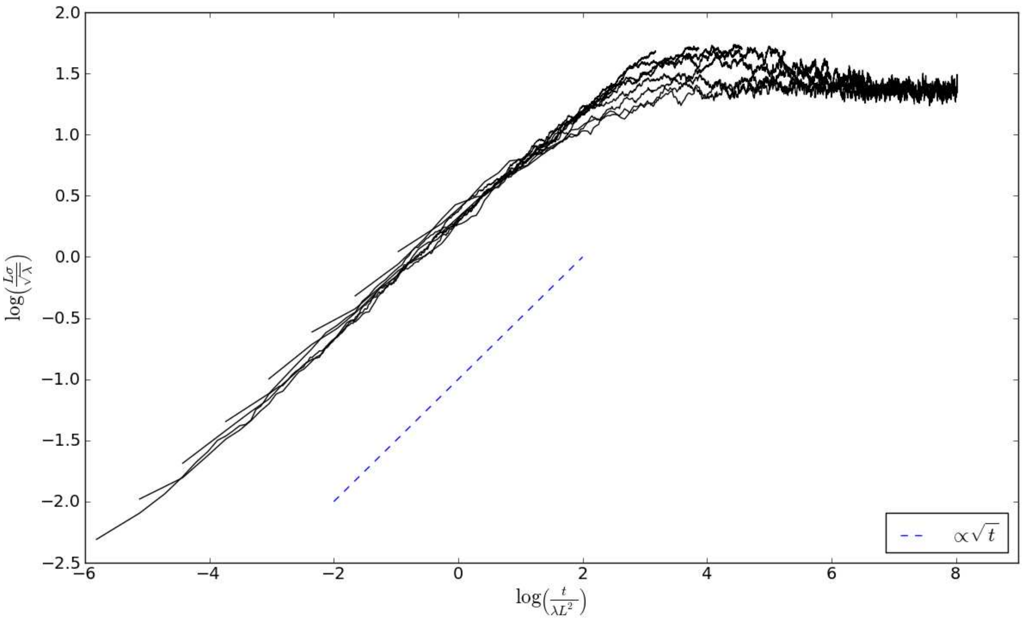


Figure 4: Graph of $\log\left(\frac{L\sigma}{\sqrt{\lambda}}\right)$ by $\log\left(\frac{t}{\lambda L^2}\right)$ for $M = 4$ and $L$ ranging from 32 to 256.

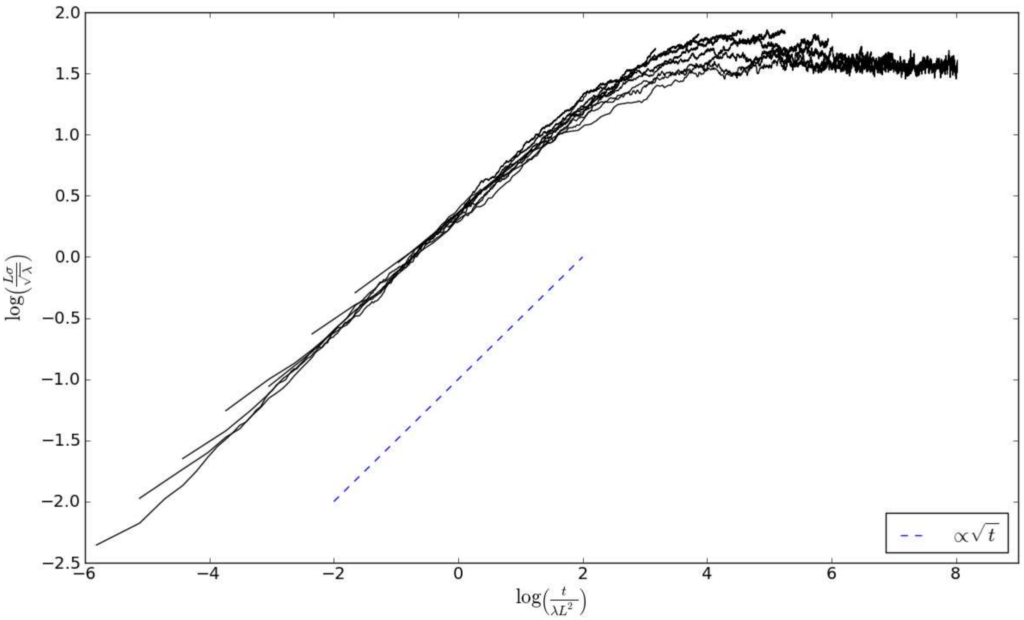


Figure 5: Graph of $\log\left(\frac{L\sigma}{\sqrt{\lambda}}\right)$ by $\log\left(\frac{t}{\lambda L^2}\right)$ for $M = 5$ and $L$ ranging from 32 to 256.

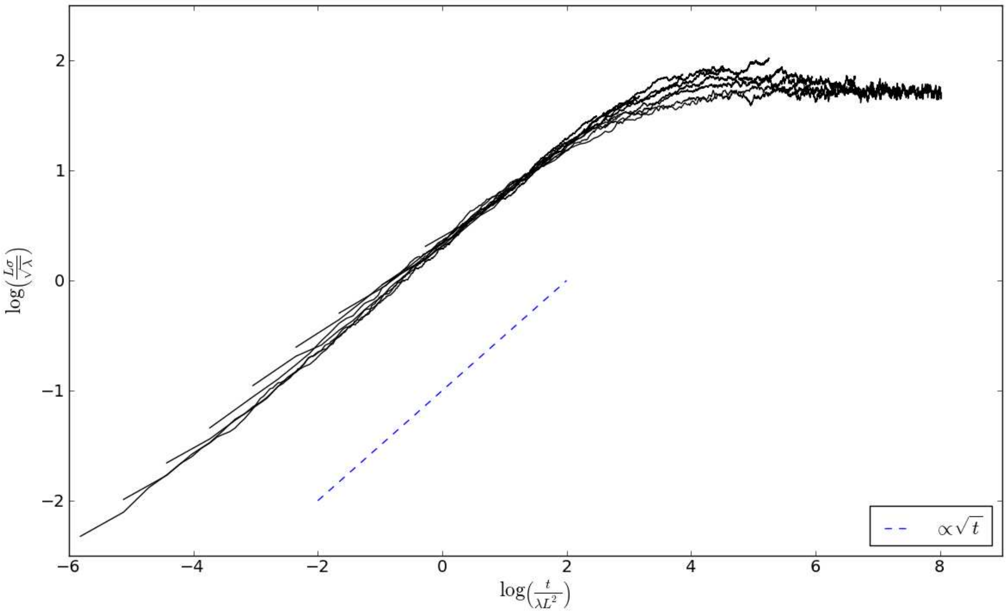


Figure 6: Graph of $\log\left(\frac{L\sigma}{\sqrt{\lambda}}\right)$ by $\log\left(\frac{t}{\lambda L^2}\right)$ for $M = 6$ and $L$ ranging from 32 to 256.

# 2 Detailed Calculations

## 2.1 Mean Field Results

One can easily write a system of mean field equations from the rules of the modified voter model

$$\begin{cases} \dot{\eta}_\sigma = -\lambda\eta_\sigma + \sum_{\sigma'\neq\sigma}(\eta_\sigma + \nu_\sigma)\nu_{\sigma'} \\ \dot{\nu}_\sigma = \lambda\eta_\sigma - \nu_\sigma \sum_{\sigma'\neq\sigma}(\eta_{\sigma'} + \nu_{\sigma'}). \end{cases} \tag{1}$$

Where $\eta_\sigma$ denotes the proportion of agents that have opinion $\sigma$ and are non-susceptibles, while $\nu_\sigma$ denotes the proportion of agents that have opinion $\sigma$ and are susceptible.

The fixed points for this system of equations can be easily found. If we define $\Delta$ as the set of surviving opinions ($\sigma \in \Delta \Leftrightarrow \eta_\sigma + \nu_\sigma \neq 0$) and $\Omega$ as the set of remaining opinions, we have one fixed point for each choice of $\Delta$:

$$\begin{cases} \nu^*_\sigma = \dfrac{\lambda}{|\Delta|\lambda + |\Delta| - 1} & \text{, if } \sigma \in \Delta \\ \eta^*_\sigma = \dfrac{|\Delta| - 1}{|\Delta|(|\Delta|\lambda + |\Delta| - 1)} & \text{, if } \sigma \in \Delta \\ \nu^*_\sigma = \eta^*_\sigma = 0 & \text{, if } \sigma \in \Omega. \end{cases} \tag{2}$$

We investigate the stability of this fixed point by evaluating the Jacobian of $\vec{F}(\vec{\eta}, \vec{\nu}) = (\dot{\vec{\eta}}, \dot{\vec{\nu}})$ at the fixed point. This leads to

$$\begin{cases} \dfrac{\partial \dot{\eta}_\sigma}{\partial \eta_{\sigma'}} = \delta_{\sigma,\sigma'}(\nu - \nu_\sigma - \lambda) \\ \dfrac{\partial \dot{\eta}_\sigma}{\partial \nu_{\sigma'}} = \delta_{\sigma,\sigma'}(\nu - 2\nu_\sigma - \eta_\sigma) + \eta_\sigma + \nu_\sigma \\ \dfrac{\partial \dot{\nu}_\sigma}{\partial \eta_{\sigma'}} = \delta_{\sigma,\sigma'}(\lambda + \nu_\sigma) - \nu_\sigma \\ \dfrac{\partial \dot{\nu}_\sigma}{\partial \nu_{\sigma'}} = \delta_{\sigma,\sigma'}(2\nu_\sigma + \eta_\sigma - 1) - \nu_\sigma \end{cases} \tag{3}$$

where

$$\nu = \sum_\sigma \nu_\sigma \Rightarrow \nu^* = \frac{\lambda|\Delta|}{|\Delta|\lambda + |\Delta| - 1} \tag{4}$$

We will write down the Jacobian evaluated in the fixed point in a block form separating variables $\eta_\sigma$ and $\nu_\sigma$ depending on whether $\sigma$ is in $\Delta$ or $\Omega$.

$$\mathcal{J}^* = \begin{bmatrix} \mathcal{J}^*_{\Delta,\Delta} & \mathcal{J}^*_{\Delta,\Omega} \\ \mathcal{J}^*_{\Omega,\Delta} & \mathcal{J}^*_{\Omega,\Omega} \end{bmatrix} \tag{5}$$

and we will write also each of the $\mathcal{J}^*_{X,Y}$ in a block form separating $\eta$ and $\nu$ variables:

$$\begin{bmatrix} \mathcal{J}^*_{\eta,\eta} & \mathcal{J}^*_{\eta,\nu} \\ \mathcal{J}^*_{\nu,\eta} & \mathcal{J}^*_{\nu,\nu} \end{bmatrix} \tag{6}$$

Substituting eq (2) in (3) implies that $\mathcal{J}^*_{\Omega,\Delta} = 0$ and

$$\mathcal{J}^*_{\Omega,\Omega} = \begin{bmatrix} (\nu^* - \lambda)\mathbb{I} & \nu^*\mathbb{I} \\ \lambda\mathbb{I} & -\mathbb{I} \end{bmatrix} \tag{7}$$

So the eigenvalues of $\mathcal{J}^*$ are the ones from $\mathcal{J}^*_{\Delta,\Delta}$ together with the ones from

$$J = \begin{bmatrix} \nu^* - \lambda & \nu^* \\ \lambda & -1 \end{bmatrix} \tag{8}$$

with multiplicity $|\Omega|$. However, substituting the solution for $\nu^*$ from eq. (4) leads to $\det(J) = \frac{-\nu^*}{|\Delta|} < 0$ meaning that $J$ has a negative and a positive eigenvalue. As a consequence all fixed points with $\Omega \neq \varnothing$ are unstable, meaning that only coexistences involving all opinions can be stable. When $\Omega = \varnothing$ then

$$\mathcal{J}^* = \mathcal{J}^*_{\Delta,\Delta} = \frac{1}{M(\lambda+\zeta)} \begin{bmatrix} -M\lambda^2\mathbb{I} & ((M-2)\lambda - \zeta)\mathbb{I} + (\lambda+\zeta)\mathbb{E} \\ \lambda(M(\lambda+\zeta)+1)\mathbb{I} - \lambda\mathbb{E} & ((2-M)\lambda + (1-M)\zeta)\mathbb{I} - \lambda\mathbb{E} \end{bmatrix} \tag{9}$$

where $\zeta = 1 - \frac{1}{M}$, $M$ is the number of opinions and $\mathbb{E} = \vec{1} \otimes \vec{1}$. The matrix in eq (9) is of the form

$$\begin{bmatrix} a\mathbb{I} + \alpha\mathbb{E} & b\mathbb{I} + \beta\mathbb{E} \\ c\mathbb{I} + \gamma\mathbb{E} & d\mathbb{I} + \delta\mathbb{E} \end{bmatrix}. \tag{10}$$

and the eigenvalues of the matrix in eq (10) are the ones from

$$J_1 = \begin{bmatrix} a & b \\ c & d \end{bmatrix}. \tag{11}$$

with multiplicity 1 and the ones from

$$J_2 = \begin{bmatrix} a + \alpha M & b + \beta M \\ c + \gamma M & d + \delta M \end{bmatrix}. \tag{12}$$

with multiplicity $M - 1$. Applying to $\mathcal{J}^*$ we have

$$J_1 = \begin{bmatrix} -M\lambda^2 & (M-2)\lambda + (M-1)\zeta + M\lambda \\ M\lambda^2 & (2-M)\lambda + (1-M)\zeta - M\lambda \end{bmatrix} \tag{13}$$

that has eigenvalues 0 and $-M(\lambda+\zeta)^2 < 0$. The null eigenvalue is an embedding artifact that comes from $\sum_\sigma(\eta_\sigma + \nu_\sigma)$ being a constant during the time evolution, meaning that it is irrelevant for the stability analysis.

$$J_2 = \begin{bmatrix} -M\lambda^2 & M\lambda - 2\lambda - \zeta \\ M\lambda^2 + M\lambda & -M\lambda + 2\lambda + \zeta - M\zeta \end{bmatrix} \tag{14}$$

Instead of calculating the eigenvalues it is easier in this case to notice that

$$\det(J_2) = M\lambda^2 + (M-1)\lambda > 0 \tag{15}$$

$$\mathrm{tr}(J_2) = 1 - \frac{3M}{4} - M\left(\lambda + \zeta - \frac{1}{2}\right)^2 < 0 \tag{16}$$

implying that both eigenvalues of $J_2$ have negative real part and hence the fixed point with $\Omega = \varnothing$ is stable. Since this fixed point is such that

$$\nu^*_\sigma + \eta^*_\sigma = \frac{1}{M} \tag{17}$$

this means that the mean-field system evolves towards a situation where all opinions are equally represented, independently of the value of $\lambda$.

## 2.2 Network Effects and Scaling Laws

To explain the finite size effects and scaling laws found in our simulations we first write a version of the mean field equations 1 that takes the lattice geometry into account:

$$\begin{cases} \dot{\eta}_\sigma = -\lambda\eta_\sigma + \left(\eta_\sigma + \nu_\sigma + \frac{L^2}{4}\nabla^2(\eta_\sigma + \nu_\sigma)\right) \sum\limits_{\sigma' \neq \sigma} \nu_{\sigma'} \\ \dot{\nu}_\sigma = \lambda\eta_\sigma + \nu_\sigma \left(\frac{L^2}{4}\nabla^2(\eta_\sigma + \nu_\sigma) - \sum\limits_{\sigma' \neq \sigma}(\eta_{\sigma'} + \nu_{\sigma'})\right) \end{cases} \tag{18}$$

and use the attractor found in section 2.1 to cast the equations in a normal form. If

$$\eta^*_\sigma = \frac{M-1}{M(\lambda M + M - 1)} \quad \text{and} \quad \nu^*_\sigma = \frac{\lambda}{\lambda M + M - 1} \tag{19}$$

then defining a perturbation $N_\sigma$ for $\eta^*_\sigma$ and $S_\sigma$ for $\nu^*_\sigma$:

$$\eta_\sigma = \eta^*_\sigma + N_\sigma \quad \text{and} \quad \nu_\sigma = \nu^*_\sigma + S_\sigma \tag{20}$$

leads to

$$\begin{cases} \dot{N}_\sigma = -\lambda N_\sigma + \frac{1}{M}\sum\limits_{\sigma' \neq \sigma} S_{\sigma'} + \frac{L^2}{4}\left(\frac{\lambda(M-1)}{\lambda M + M - 1} + \sum\limits_{\sigma' \neq \sigma} S_{\sigma'}\right)\nabla^2(N_\sigma + S_\sigma) \\ \dot{S}_\sigma = \lambda N_\sigma + \left(\frac{\lambda}{\lambda M + M - 1} + S_\sigma\right)\left(N_\sigma + S_\sigma + \frac{L^2}{4}\nabla^2(N_\sigma + S_\sigma)\right) - S_\sigma\frac{(M-1)}{M} \end{cases} \tag{21}$$

where we have rescaled the lattice size to 1 (hence the appearance of the $L^2\nabla^2$ operators)

Taking $\lambda \gg 1$ and $N_\sigma, S_\sigma \ll 1$ (and defining $\Theta_\sigma = N_\sigma + S_\sigma$) we can approximate the equations for the perturbations $N$ and $S$ as

$$\begin{cases} \dot{N}_\sigma = -\lambda N_\sigma + \frac{L^2(M-1)}{4M}\nabla^2(N_\sigma + S_\sigma) \\ \dot{S}_\sigma = \lambda N_\sigma + \frac{L^2}{4M}\nabla^2(N_\sigma + S_\sigma) \end{cases} \tag{22}$$

$$\begin{cases} \dot{N}_\sigma = -\lambda N_\sigma + \frac{L^2}{4}\nabla^2\Theta_\sigma \\ \dot{\Theta}_\sigma = \lambda N_\sigma + \frac{L^2(M-1)}{4M}\nabla^2\Theta_\sigma \end{cases} \tag{23}$$

These equations give a normal form for the lattice equations and as shown in the main article, allow us to tell how spatial patterns will scale with $L$ and $\lambda$.
